# Supplementary material for: Goldilocks: Consistent Crowdsourced Scalar Annotations with Relative Uncertainty
Source: arXiv:2108.01799 source file (2021-08-04)
Supplement: Supplementary file 1 [file s_appendix.tex]

\appendix

\section{This is the appendix}

Placeholder
